# Supplementary material for: Transient dynamics of subradiance and superradiance in open optical ensembles
Source: arXiv:2205.06319 ancillary file (2023-03-10)
Supplement: Supplementary file 1 [file PRL2022_supplement.pdf]

## RADIATED FIELD IN ROTATING FRAME

Start from the single dot Hamiltonian:

$$\mathcal{H}(t) = \begin{pmatrix} 0 & -\hbar\chi(t) \\ -\hbar\chi^*(t) & \hbar\omega \end{pmatrix} \quad (1)$$

and its rotating frame representation ( $U = \text{diag}(1, e^{i\omega_L t})$ ):

$$\tilde{\mathcal{H}}(t) = U\mathcal{H}U^\dagger - i\hbar U\dot{U}^\dagger = \begin{pmatrix} 0 & -\hbar\chi(t)e^{-i\omega_L t} \\ -\hbar\chi^*(t)e^{i\omega_L t} & \hbar(\omega - \omega_L) \end{pmatrix} \quad (2)$$

The rotating frame Liouville equations  $\hbar\dot{\rho}^i = -i[\tilde{\mathcal{H}}^i(t), \tilde{\rho}^i] - \mathcal{D}[\tilde{\rho}^i]$  take the form:

$$\begin{cases} \dot{\rho}_{00} = -i(\tilde{\chi}\tilde{\rho}_{01}^* - \tilde{\chi}^*\tilde{\rho}_{01}) - (\tilde{\rho}_{00} - 1)/T_1 \\ \dot{\rho}_{01} = -i(\tilde{\chi}(1 - 2\tilde{\rho}_{00}) + \tilde{\rho}_{01}(\omega_L - \omega)) - \tilde{\rho}_{01}/T_2 \end{cases} \quad (3)$$

where  $\tilde{\chi} = \chi e^{-i\omega_L t} = \mathbf{d} \cdot (\tilde{\mathbf{E}}_L + \tilde{\mathfrak{F}}\{\mathbf{P}\})/\hbar$ . We may assume the Rotating Wave Approximation (RWA) for our polarization  $\mathbf{P} = \tilde{\rho}_{01}\mathbf{d}e^{i\omega_L t} = \tilde{\mathbf{P}}e^{i\omega_L t}$ . The rotating frame radiated field takes the form (cf. (1)):

$$\begin{aligned} \tilde{\mathfrak{F}}\{\tilde{\mathbf{P}}(\mathbf{r}, t)\} = & \frac{-1}{4\pi\epsilon} \int \left[ (\mathbf{I} - \bar{\mathbf{r}} \otimes \bar{\mathbf{r}}) \cdot \frac{\partial_t^2 \tilde{\mathbf{P}} + 2i\omega_L \partial_t \tilde{\mathbf{P}} - \omega_L^2 \tilde{\mathbf{P}}}{c^2 R} + \right. \\ & \left. + (\mathbf{I} - 3\bar{\mathbf{r}} \otimes \bar{\mathbf{r}}) \cdot \left( \frac{\partial_t \tilde{\mathbf{P}} + i\omega_L \tilde{\mathbf{P}}}{cR^2} + \frac{\tilde{\mathbf{P}}}{R^3} \right) \right] e^{-ikR} d^3\mathbf{r}' \end{aligned} \quad (4)$$

where  $k = \omega_L/c$ ,  $t_R = t - R/c$ , and  $\tilde{\mathbf{P}} = \tilde{\mathbf{P}}(\mathbf{r}', t_R)$ . The radiated field Rabi frequency then separates as  $\chi_{Rad} = \hat{\mathbf{d}} \cdot \tilde{\mathfrak{F}}\{\tilde{\mathbf{P}}\}/\hbar = -(\Omega + i\gamma)$ , where:

$$\begin{aligned} \Omega(\mathbf{r}, t) \approx & \frac{3}{4}\Gamma \left\{ \rho_{01,r} \left( -(I - \hat{\mathbf{r}} \otimes \hat{\mathbf{r}}) \frac{\cos kR}{kR} + (I - 3\hat{\mathbf{r}} \otimes \hat{\mathbf{r}}) \left( \frac{\sin kR}{(kR)^2} + \frac{\cos kR}{(kR)^3} \right) \right) \right. \\ & \left. + \rho_{01,i} \left( -(I - \hat{\mathbf{r}} \otimes \hat{\mathbf{r}}) \frac{\sin kR}{kR} + (I - 3\hat{\mathbf{r}} \otimes \hat{\mathbf{r}}) \left( -\frac{\cos kR}{(kR)^2} + \frac{\sin kR}{(kR)^3} \right) \right) \right\} \end{aligned} \quad (5)$$

$$\begin{aligned} \gamma(\mathbf{r}, t) \approx & \frac{3}{4}\Gamma \left\{ \rho_{01,r} \left( (I - \hat{\mathbf{r}} \otimes \hat{\mathbf{r}}) \frac{\sin kR}{kR} + (I - 3\hat{\mathbf{r}} \otimes \hat{\mathbf{r}}) \left( \frac{\cos kR}{(kR)^2} + \frac{\sin kR}{(kR)^3} \right) \right) \right. \\ & \left. + \rho_{01,i} \left( -(I - \hat{\mathbf{r}} \otimes \hat{\mathbf{r}}) \frac{\cos kR}{kR} + (I - 3\hat{\mathbf{r}} \otimes \hat{\mathbf{r}}) \left( \frac{\sin kR}{(kR)^2} + \frac{\cos kR}{(kR)^3} \right) \right) \right\} \end{aligned} \quad (6)$$

and  $\Gamma = d^2\omega_L^3/3\pi\epsilon\hbar c^3$  is the spontaneous decay rate for this emitter. (For brevity we have disregarded the derivative terms, as they have a similar spatial dependence as the terms shown above.)

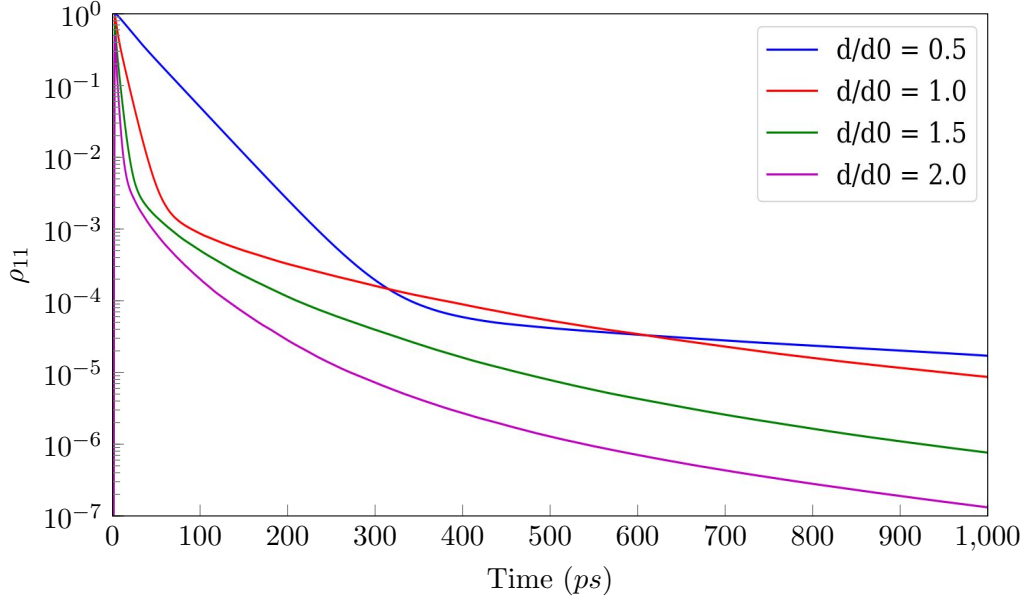

SUPPLEMENTARY FIG. 1. Time evolution of space-averaged population excitation  $\rho_{11}$ , corresponding to Fig. 1. Shown are dot-averaged values for  $N = 200$  at various dipole strengths.

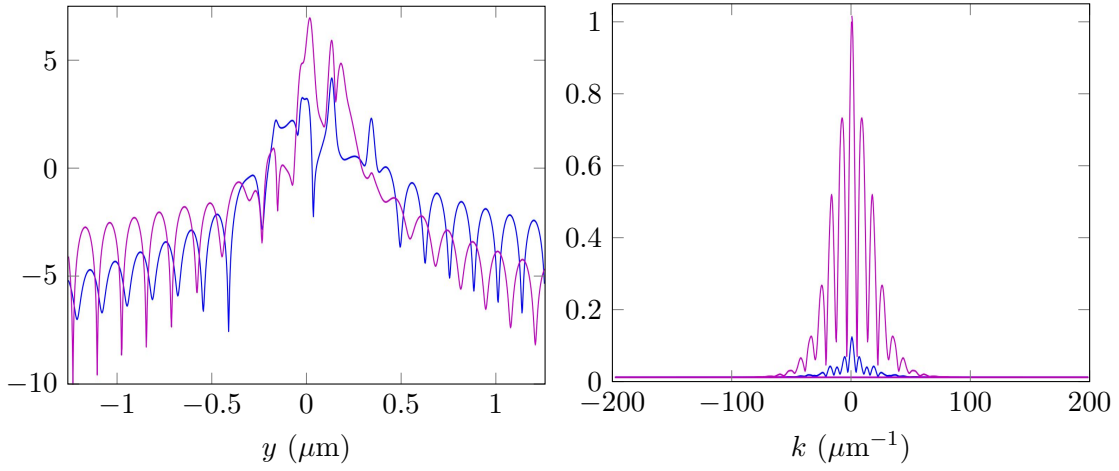

SUPPLEMENTARY FIG. 2. Plot of logarithmic field intensity (Left) and its Fourier transform (Right) along the  $y$  axis for  $d/d_0 = 1.0$  (Blue) and  $d/d_0 = 2.0$  (Magenta), corresponding to Fig. 3 (a). The Fourier data is normalized against the  $d/d_0 = 2.0$  series.

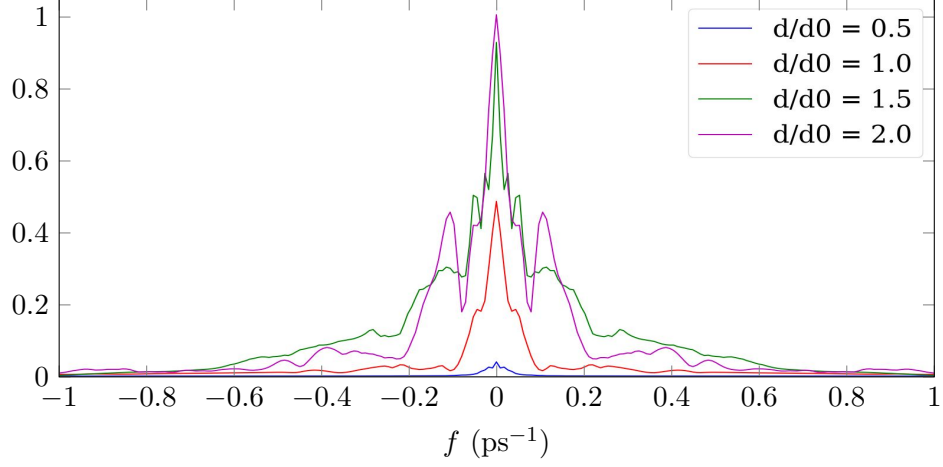

SUPPLEMENTARY FIG. 3. Temporal Fourier plot of logarithmic field intensity along the  $y$  axis (Fig. 4) for  $N = 200$  and various dipole strengths. Spectral broadening with increasing dipole strength is evident.

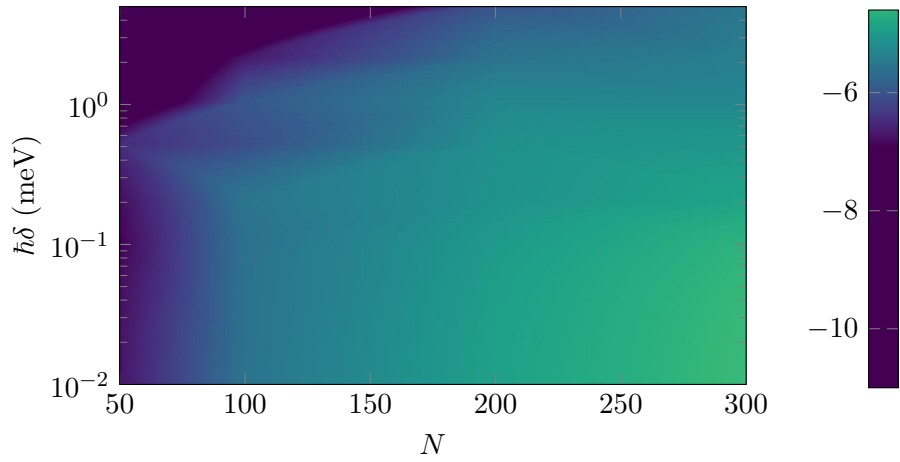

SUPPLEMENTARY FIG. 4. Phase space plot of averaged steady population inversion as a function of inhomogeneous broadening  $\delta$  and  $N$  for  $d/d_0 = 1.0$ .
